# Supplementary material for: Prototypical Fine-tuning: Towards Robust Performance Under Varying Data Sizes
Source: arXiv:2211.13638 source file (2022-11-24)
Supplement: Supplementary file 1 [file supplementary.tex]

\subsection{Extension}

\begin{table}
\small
\addtolength{\tabcolsep}{-2pt}
\begin{tabular}{l|ccccccccc} 
\hline
\hline
Model                            & MNLI-m                  & MNLI-mm                 & QQP                         & QNLI                     & SST-2                    & CoLA                     & STS-B                   & MRPC                        & RTE                      \\ 
\hline
$\operatorname{BERT_{Base}}$     & 83.6                    & 83.8                    & 90.2/86.7                   & 90.7                     & 93.4                     & 56.2                     & 87.9                    & 83.6/88.5                   & 70.4                     \\
~~ + PFit                        & \textbf{84.2}           & \textbf{84.3}           & \textbf{90.8}/\textbf{87.7} & \textbf{91.3}            & \textbf{93.9}            & \textbf{58.9}            & \textbf{89.2}           & \textbf{87.0/89.2}          & \textbf{72.5}            \\
\textit{Impr.}                         & {0.6} & {0.5} & {0.6/1.0} & {0.6}  & {0.5}  & {2.7}  & {1.3} & {3.4/0.7} & {2.1}  \\ 
\hline
$\operatorname{BERT_{Large}}$    & 86.5                    & 86.7                    & 90.3/86.9                   & 93.0                     & 94.0                     & 59.7                     & 89.8                    & 87.5/91.1                   & 71.5                     \\
~~ + PFit                        & \textbf{87.0}           & \textbf{87.1}           & \textbf{90.8}/\textbf{87.8} & \textbf{93.2}            & \textbf{94.4}            & \textbf{60.0}            & \textbf{90.3}           & \textbf{88.2}/\textbf{91.5} & \textbf{74.8}            \\
\textit{Impr.}                       & {0.5} & {0.4} & {0.5/0.9} & {0.2}  & {0.4}  & {0.3}  & {0.5} & {0.7/0.4} & {3.3}  \\ 
\hline
$\operatorname{RoBERTa_{Base}}$  & 87.4                    & 87.4                    & 91.3/88.7                   & 93.0                     & 94.5                     & 61.1                     & 90.5                    & 87.2/90.8                   & 77.1                     \\
~~ + PFit                        & \textbf{87.6}           & \textbf{87.8}           & \textbf{91.7}/\textbf{88.9} & \textbf{93.3}            & \textbf{94.9}            & \textbf{62.9}            & \textbf{91.1}           & \textbf{88.8}/\textbf{92.0} & \textbf{83.2}            \\
\textit{Impr.}                       & {0.2} & {0.4} & {0.4/0.3} & {0.2}  & {0.4}  & {1.8}  & {0.6} & {1.6/1.2} & {6.1}  \\ 
\hline
$\operatorname{RoBERTa_{Large}}$ & 90.3                    & 90.4                    & 92.0/88.3                   & 94.6                     & 95.8                     & 66.5                     & 92.1                    & 89.5/92.5                   & 83.5                     \\
~~ + PFit                        & \textbf{90.7}           & \textbf{90.7}           & \textbf{92.5}/\textbf{89.6} & 94.6                     & \textbf{96.1}            & \textbf{67.8}            & \textbf{92.4}           & \textbf{89.7}/\textbf{93.2} & \textbf{84.6}            \\
\textit{Impr.}                       & {0.4} & {0.3} & {0.5/1.3} & 0.0    & {0.3}  & {1.3}  & {0.3} & {0.2/0.7} & {1.1}  \\ 
\hline
$\operatorname{ELECTRA_{Small}}$ & 81.2                    & 81.5                    & 89.1/87.2                   & \textbf{88.4}            & 91.1                     & \textbf{57.0}            & 87.5                    & 87.8/88.3                   & 66.7                     \\
~~ + PFit                        & 81.2                    & \textbf{82.0}           & \textbf{90.5}/\textbf{89.2} & \textbf{88.7}              & 91.1                     & 56.7                     & \textbf{88.0}           & \textbf{87.9}/\textbf{88.7} & \textbf{73.8}            \\
\textit{Impr.}                       & 0.0   & {0.5} & {1.4/2.0} & 0.3 & {0.0}  & {-0.3} & {0.5} & {0.1/0.4} & {7.1}  \\ 
\hline
$\operatorname{ELECTRA_{Base}}$  & 88.5                    & 88.8                    & 91.7/89.1                   & 93.1                     & \textbf{95.4}            & 67.3                     & 91.2                    & 88.2/\textbf{91.6}          & 82.4                     \\
~~ + PFit                        & \textbf{89.0}           & \textbf{89.2}           & \textbf{92.2}/\textbf{89.5} & 93.1                     & 95.3                     & \textbf{68.3}            & \textbf{91.8}           & 88.2/91.3                   & \textbf{82.6}            \\
\textit{Impr.}                       & {0.5} & {0.4} & {0.5/0.4} & 0.0 & {-0.1} & {1.0}  & {0.6} & {0.0/0.3}   & {0.2}  \\
\hline
\hline
% \label{fig:full}
\end{tabular}
\vspace{1mm}
\caption{Performance comparison of 6 original language models and PFit on the GLUE benchmark. PFit can reach comparable and usually better performances than the vanilla LMs.}
\label{fig:full}
\vspace{-1mm}
\end{table}

\textbf{Multi-label classification}

\subsection{Discussion}

\textbf{Relation to Prompt-tuning}

Prompt-tuning focuses more on the parameter efficiency, and the performances are generally worse than the original model~\cite{lester2021power}. Prompt-tuning adds extra tunable token embeddings on the input, while the original parameters are frozen. The effectiveness of prompt learning is constrained by how conditioning text can fit into the model's input~\cite{lester2021power}.

Prototypical learning has a stronger emphasis on performance improvement. Under prototypical learning, the parameters of the base models are updating, in contrast to prompt-tuning. They can achieve superior performances across a wide spectrum of classification and regression tasks, especially under low-resource settings. In particular, our approach can adaptively adjust its capacity to different distributions of data, and constantly outperforms all other baselines across a variety of tasks on low-resource settings.

\subsection{Stronger Regularization}

In Tab.~\ref{fig:sam}, we experimented with the effect of stronger regularization~\cite{foret2020sharpness}, which does not lead to statistically significant improvements in the performances.

\begin{figure}
\vspace{-1mm}
\begin{center}
\includegraphics[width=0.43 \textwidth]{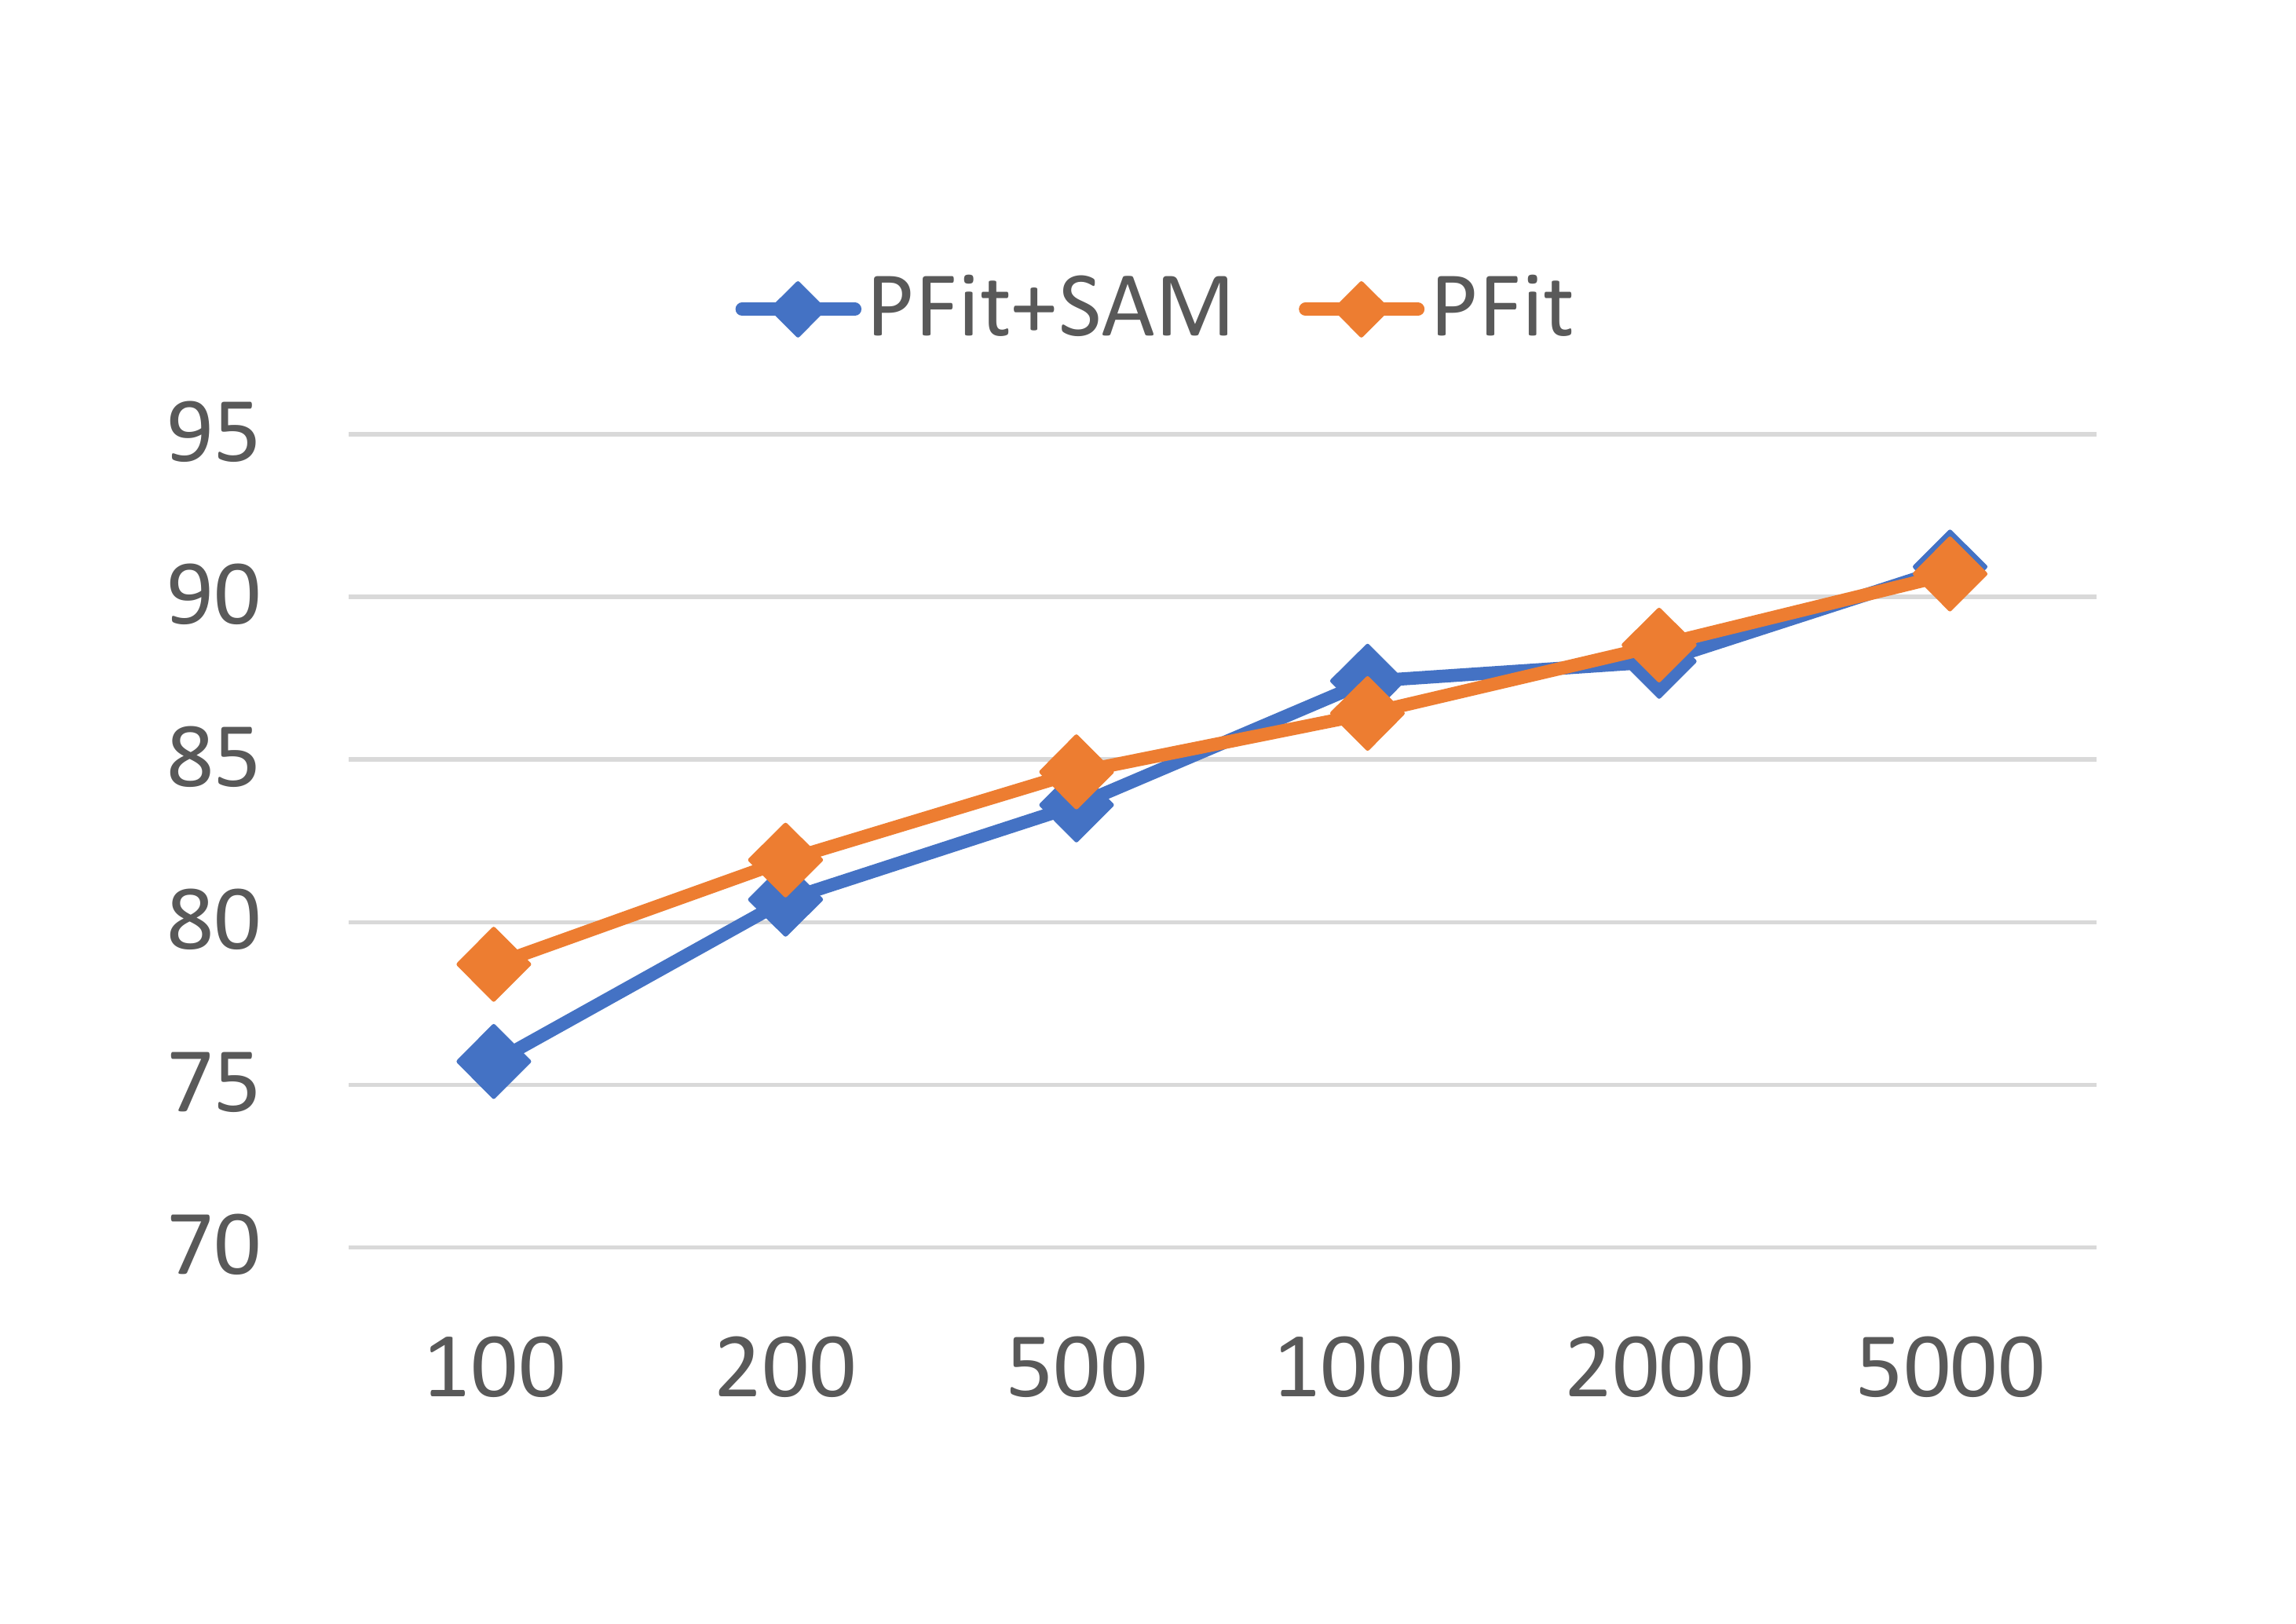}
\end{center}
\vspace{-3mm}
\caption{Performance of PFit and PFit with Sharpness Aware Minimization (PFit+SAM)}
\label{fig:sam}
\vspace{-3mm}
\end{figure}

\subsubsection{Sensitivity Analysis}
We investigate the size of the sliding window $\delta$ towards the model's accuracy and the end-of-training prototype number as in Table~\ref{fig:sensitivity}. We observe that the accuracy is positively correlated with $\delta$ and negatively correlated with the number of prototypes. It is possible that a small number of $\delta$ examples cannot sufficiently validate the representativeness of prototype vectors and can hamper the pruning of less meaningful prototypes.
Although a larger $\delta$ generally leads to better accuracy, setting $\delta = 800$ is sufficient for ensuring performance.

\begin{figure}
\vspace{-1mm}
\begin{center}
\includegraphics[width=0.43 \textwidth]{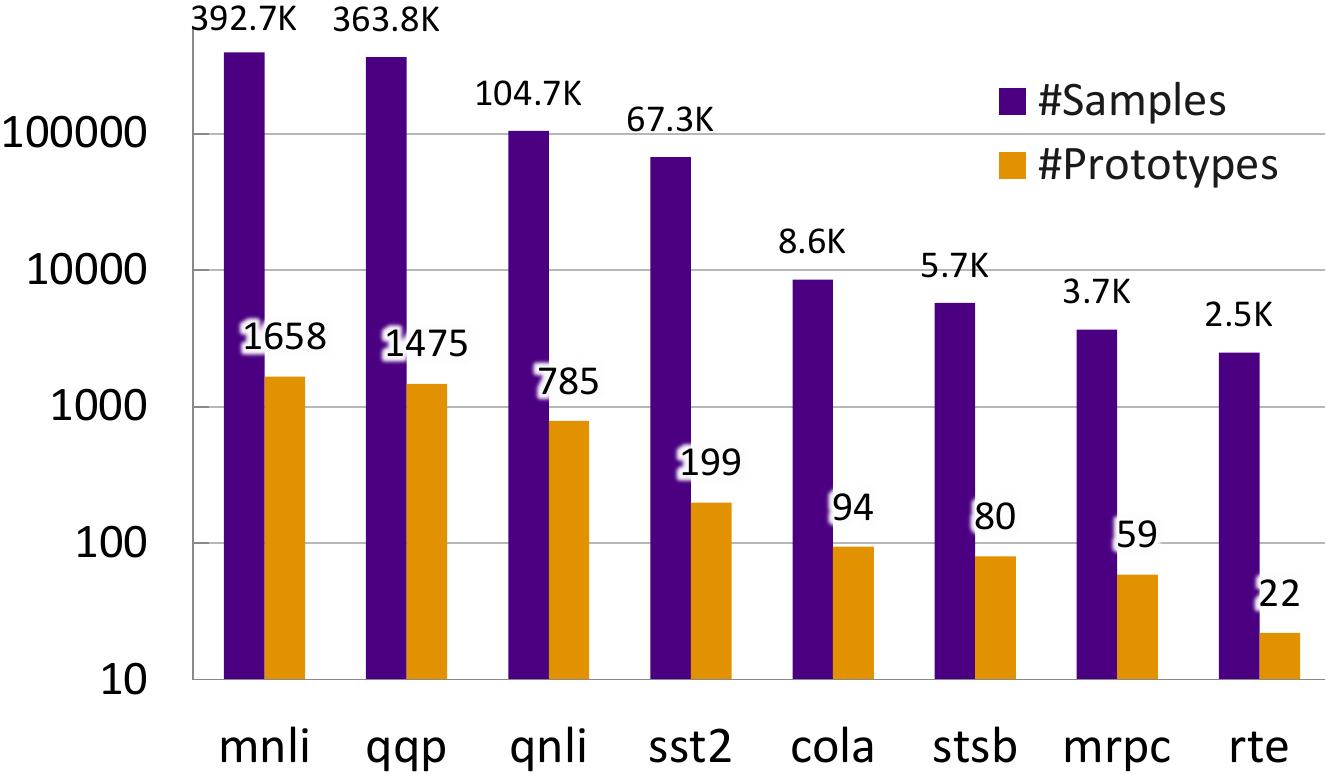}
\end{center}
\vspace{-3mm}
\caption{Number of prototypes created by PFit on each dataset of GLUE benchmark.}
\label{fig:num_protos}
\vspace{-3mm}
\end{figure}
% ---------------

\subsection{Adaptive Capacity} Fig.~\ref{fig:num_protos} shows the number of generated prototypes on each dataset of GLUE. Although the number of prototypes do not necessarily follow a linear relationship with data sizes, a greater number of prototypes usually corresponds to a larger dataset. Our results demonstrate the adaptability and scalability of PFit as it is able to model datasets with varying sizes and complexity.

\subsubsection{High-Resource Settings}
We evaluate the performances in high-resource settings with 6 pretrained models including 2 variations of BERT~\cite{devlin2019bert}, RoBERTa~\cite{liu2019roberta}, and ELECTRA~\cite{clark2019electra}, respectively. 
% As we enlarge the fine-tuning datasets, performances of raw models gradually approach PFit. 
For full dataset, our prototypical models can achieve comparable and usually better performances compared to the raw models. Overall, our results demonstrate that our proposed PFit model is effective across varying data sizes.

\subsection{Discussion}

\subsubsection{Limitation}

\subsubsection{Broader Impact}

Many language models exhibit socially problematic biases derived from the pretraining corpora~\cite{bordia2019identifying}. Due to the mechanism of prototypical networks, although our method may reflect these biases through prototype embeddings and predictions, it can also serve to pinpoint, explain, and correct these biases.
